# Supplementary material for: Minimal complete sets for two pseudoscalar meson photoproduction
Source: arXiv:2009.04356 ancillary file (2020-10-27)
Supplement: Supplementary file 1 [file supplement.pdf]

# Supplementary material for the paper 'Minimal complete sets for two pseudoscalar meson photoproduction'

Philipp Kroenert,[1] Yannick Wunderlich,[1] Farah Afzal,[1] and Annika Thiel[1]
[1] *Helmholtz Institut für Strahlen- und Kernphysik, Universität Bonn, Germany*

## I. ALGEBRAIC REDUCTION TO MINIMAL COMPLETE SETS

It is also possible to deduce complete sets of $2N = 16$ observables using algebraic methods. In the following, the phase-fixing approach first developed by Nakayama in a treatment of single-meson photoproduction (i.e. for $N = 4$ amplitudes) [1] is extended to 2-meson photoproduction. The approach described in section IV of reference [1] has been used as a logical starting point in order to deduce the procedure described in the following.

Much of the algebraic approach rests on the possibility to "decouple" the seven non-diagonal shape-classes of observables collected in Tables I and II of the main paper. This works as follows: for any shape-class $n \in \{\mathrm{II}, \ldots, \mathrm{VIII}\}$, the associated decoupled "$a$-class" is defined via the sums:

$$\tilde{\mathcal{O}}^{n\mathrm{a}}_{1+} := \frac{1}{2}\left(\mathcal{O}^{n}_{s1} + \mathcal{O}^{n}_{s2}\right), \tag{1}$$

$$\tilde{\mathcal{O}}^{n\mathrm{a}}_{1-} := \frac{1}{2}\left(\mathcal{O}^{n}_{s3} + \mathcal{O}^{n}_{s4}\right), \tag{2}$$

$$\tilde{\mathcal{O}}^{n\mathrm{a}}_{2+} := \frac{1}{2}\left(\mathcal{O}^{n}_{c1} + \mathcal{O}^{n}_{c2}\right), \tag{3}$$

$$\tilde{\mathcal{O}}^{n\mathrm{a}}_{2-} := \frac{1}{2}\left(\mathcal{O}^{n}_{c3} + \mathcal{O}^{n}_{c4}\right), \tag{4}$$

and the associated decoupled '$b$-class' is defined by the following differences:

$$\tilde{\mathcal{O}}^{n\mathrm{b}}_{1+} := \frac{1}{2}\left(\mathcal{O}^{n}_{s1} - \mathcal{O}^{n}_{s2}\right), \tag{5}$$

$$\tilde{\mathcal{O}}^{n\mathrm{b}}_{1-} := \frac{1}{2}\left(\mathcal{O}^{n}_{s3} - \mathcal{O}^{n}_{s4}\right), \tag{6}$$

$$\tilde{\mathcal{O}}^{n\mathrm{b}}_{2+} := \frac{1}{2}\left(\mathcal{O}^{n}_{c1} - \mathcal{O}^{n}_{c2}\right), \tag{7}$$

$$\tilde{\mathcal{O}}^{n\mathrm{b}}_{2-} := \frac{1}{2}\left(\mathcal{O}^{n}_{c3} - \mathcal{O}^{n}_{c4}\right). \tag{8}$$

As an example, the results for the decoupled shape-class IIa is listed:

$$\tilde{\mathcal{O}}^{\mathrm{IIa}}_{1+} = |t_1|\,|t_3| \sin\phi_{13} + |t_2|\,|t_4| \sin\phi_{24}, \tag{9}$$

$$\tilde{\mathcal{O}}^{\mathrm{IIa}}_{1-} = |t_1|\,|t_3| \sin\phi_{13} - |t_2|\,|t_4| \sin\phi_{24}, \tag{10}$$

$$\tilde{\mathcal{O}}^{\mathrm{IIa}}_{2+} = |t_1|\,|t_3| \cos\phi_{13} + |t_2|\,|t_4| \cos\phi_{24}, \tag{11}$$

$$\tilde{\mathcal{O}}^{\mathrm{IIa}}_{2-} = |t_1|\,|t_3| \cos\phi_{13} - |t_2|\,|t_4| \cos\phi_{24}, \tag{12}$$

as well as for class IIb:

$$\tilde{\mathcal{O}}^{\mathrm{IIb}}_{1+} = |t_5|\,|t_7| \sin\phi_{57} + |t_6|\,|t_8| \sin\phi_{68}, \tag{13}$$

$$\tilde{\mathcal{O}}^{\mathrm{IIb}}_{1-} = |t_5|\,|t_7| \sin\phi_{57} - |t_6|\,|t_8| \sin\phi_{68}. \tag{14}$$

$$\tilde{\mathcal{O}}^{\mathrm{IIb}}_{2+} = |t_5|\,|t_7| \cos\phi_{57} + |t_6|\,|t_8| \cos\phi_{68}, \tag{15}$$

$$\tilde{\mathcal{O}}^{\mathrm{IIb}}_{2-} = |t_5|\,|t_7| \cos\phi_{57} - |t_6|\,|t_8| \cos\phi_{68}. \tag{16}$$

These 2 "photoproduction-like" shape-classes just have the same algebraic structure than what is written, for instance, in Table IV of [2]. Therefore, the same notation is re-introduced for the observables as used in the Nakayama-paper [1].

It is clear that what has been done for the original shape-class "II" can be repeated in the same way, with very similar equations, for the remaining shape-classes "III" to "VIII" defined in the main paper. The results are shown in

TABLE I. The results for the decoupling of shape-classes are collected here for the classes "II", "III", "IV" and "V". The corresponding relative phases are indicated on the right.

| Observable | (Shape-) class | Relative phases |
|---|---|---|
| $\tilde{\mathcal{O}}^{\mathrm{IIa}}_{1+} := \frac{1}{2}\left(\mathcal{O}^{\mathrm{II}}_{s,1} + \mathcal{O}^{\mathrm{II}}_{s,2}\right) = \left|t_1\right| \left|t_3\right| \sin\phi_{13} + \left|t_2\right| \left|t_4\right| \sin\phi_{24}$ | | |
| $\tilde{\mathcal{O}}^{\mathrm{IIa}}_{1-} := \frac{1}{2}\left(\mathcal{O}^{\mathrm{II}}_{s,3} + \mathcal{O}^{\mathrm{II}}_{s,4}\right) = \left|t_1\right| \left|t_3\right| \sin\phi_{13} - \left|t_2\right| \left|t_4\right| \sin\phi_{24}$ | IIa | $\{\phi_{13}, \phi_{24}\}$ |
| $\tilde{\mathcal{O}}^{\mathrm{IIa}}_{2+} := \frac{1}{2}\left(\mathcal{O}^{\mathrm{II}}_{c,1} + \mathcal{O}^{\mathrm{II}}_{c,2}\right) = \left|t_1\right| \left|t_3\right| \cos\phi_{13} + \left|t_2\right| \left|t_4\right| \cos\phi_{24}$ | | |
| $\tilde{\mathcal{O}}^{\mathrm{IIa}}_{2-} := \frac{1}{2}\left(\mathcal{O}^{\mathrm{II}}_{c,3} + \mathcal{O}^{\mathrm{II}}_{c,4}\right) = \left|t_1\right| \left|t_3\right| \cos\phi_{13} - \left|t_2\right| \left|t_4\right| \cos\phi_{24}$ | | |
| $\tilde{\mathcal{O}}^{\mathrm{IIb}}_{1+} := \frac{1}{2}\left(\mathcal{O}^{\mathrm{II}}_{s,1} - \mathcal{O}^{\mathrm{II}}_{s,2}\right) = \left|t_5\right| \left|t_7\right| \sin\phi_{57} + \left|t_6\right| \left|t_8\right| \sin\phi_{68}$ | | |
| $\tilde{\mathcal{O}}^{\mathrm{IIb}}_{1-} := \frac{1}{2}\left(\mathcal{O}^{\mathrm{II}}_{s,3} - \mathcal{O}^{\mathrm{II}}_{s,4}\right) = \left|t_5\right| \left|t_7\right| \sin\phi_{57} - \left|t_6\right| \left|t_8\right| \sin\phi_{68}$ | IIb | $\{\phi_{57}, \phi_{68}\}$ |
| $\tilde{\mathcal{O}}^{\mathrm{IIb}}_{2+} := \frac{1}{2}\left(\mathcal{O}^{\mathrm{II}}_{c,1} - \mathcal{O}^{\mathrm{II}}_{c,2}\right) = \left|t_5\right| \left|t_7\right| \cos\phi_{57} + \left|t_6\right| \left|t_8\right| \cos\phi_{68}$ | | |
| $\tilde{\mathcal{O}}^{\mathrm{IIb}}_{2-} := \frac{1}{2}\left(\mathcal{O}^{\mathrm{II}}_{c,3} - \mathcal{O}^{\mathrm{II}}_{c,4}\right) = \left|t_5\right| \left|t_7\right| \cos\phi_{57} - \left|t_6\right| \left|t_8\right| \cos\phi_{68}$ | | |
| $\tilde{\mathcal{O}}^{\mathrm{IIIa}}_{1+} := \frac{1}{2}\left(\mathcal{O}^{\mathrm{III}}_{s,1} + \mathcal{O}^{\mathrm{III}}_{s,2}\right) = \left|t_1\right| \left|t_2\right| \sin\phi_{12} + \left|t_3\right| \left|t_4\right| \sin\phi_{34}$ | | |
| $\tilde{\mathcal{O}}^{\mathrm{IIIa}}_{1-} := \frac{1}{2}\left(\mathcal{O}^{\mathrm{III}}_{s,3} + \mathcal{O}^{\mathrm{III}}_{s,4}\right) = \left|t_1\right| \left|t_2\right| \sin\phi_{12} - \left|t_3\right| \left|t_4\right| \sin\phi_{34}$ | IIIa | $\{\phi_{12}, \phi_{34}\}$ |
| $\tilde{\mathcal{O}}^{\mathrm{IIIa}}_{2+} := \frac{1}{2}\left(\mathcal{O}^{\mathrm{III}}_{c,1} + \mathcal{O}^{\mathrm{III}}_{c,2}\right) = \left|t_1\right| \left|t_2\right| \cos\phi_{12} + \left|t_3\right| \left|t_4\right| \cos\phi_{34}$ | | |
| $\tilde{\mathcal{O}}^{\mathrm{IIIa}}_{2-} := \frac{1}{2}\left(\mathcal{O}^{\mathrm{III}}_{c,3} + \mathcal{O}^{\mathrm{III}}_{c,4}\right) = \left|t_1\right| \left|t_2\right| \cos\phi_{12} - \left|t_3\right| \left|t_4\right| \cos\phi_{34}$ | | |
| $\tilde{\mathcal{O}}^{\mathrm{IIIb}}_{1+} := \frac{1}{2}\left(\mathcal{O}^{\mathrm{III}}_{s,1} - \mathcal{O}^{\mathrm{III}}_{s,2}\right) = \left|t_5\right| \left|t_6\right| \sin\phi_{56} + \left|t_7\right| \left|t_8\right| \sin\phi_{78}$ | | |
| $\tilde{\mathcal{O}}^{\mathrm{IIIb}}_{1-} := \frac{1}{2}\left(\mathcal{O}^{\mathrm{III}}_{s,3} - \mathcal{O}^{\mathrm{III}}_{s,4}\right) = \left|t_5\right| \left|t_6\right| \sin\phi_{56} - \left|t_7\right| \left|t_8\right| \sin\phi_{78}$ | IIIb | $\{\phi_{56}, \phi_{78}\}$ |
| $\tilde{\mathcal{O}}^{\mathrm{IIIb}}_{2+} := \frac{1}{2}\left(\mathcal{O}^{\mathrm{III}}_{c,1} - \mathcal{O}^{\mathrm{III}}_{c,2}\right) = \left|t_5\right| \left|t_6\right| \cos\phi_{56} + \left|t_7\right| \left|t_8\right| \cos\phi_{78}$ | | |
| $\tilde{\mathcal{O}}^{\mathrm{IIIb}}_{2-} := \frac{1}{2}\left(\mathcal{O}^{\mathrm{III}}_{c,3} - \mathcal{O}^{\mathrm{III}}_{c,4}\right) = \left|t_5\right| \left|t_6\right| \cos\phi_{56} - \left|t_7\right| \left|t_8\right| \cos\phi_{78}$ | | |
| $\tilde{\mathcal{O}}^{\mathrm{IVa}}_{1+} := \frac{1}{2}\left(\mathcal{O}^{\mathrm{IV}}_{s,1} + \mathcal{O}^{\mathrm{IV}}_{s,2}\right) = \left|t_1\right| \left|t_4\right| \sin\phi_{14} + \left|t_2\right| \left|t_3\right| \sin\phi_{23}$ | | |
| $\tilde{\mathcal{O}}^{\mathrm{IVa}}_{1-} := \frac{1}{2}\left(\mathcal{O}^{\mathrm{IV}}_{s,3} + \mathcal{O}^{\mathrm{IV}}_{s,4}\right) = \left|t_1\right| \left|t_4\right| \sin\phi_{14} - \left|t_2\right| \left|t_3\right| \sin\phi_{23}$ | IVa | $\{\phi_{14}, \phi_{23}\}$ |
| $\tilde{\mathcal{O}}^{\mathrm{IVa}}_{2+} := \frac{1}{2}\left(\mathcal{O}^{\mathrm{IV}}_{c,1} + \mathcal{O}^{\mathrm{IV}}_{c,2}\right) = \left|t_1\right| \left|t_4\right| \cos\phi_{14} + \left|t_2\right| \left|t_3\right| \cos\phi_{23}$ | | |
| $\tilde{\mathcal{O}}^{\mathrm{IVa}}_{2-} := \frac{1}{2}\left(\mathcal{O}^{\mathrm{IV}}_{c,3} + \mathcal{O}^{\mathrm{IV}}_{c,4}\right) = \left|t_1\right| \left|t_4\right| \cos\phi_{14} - \left|t_2\right| \left|t_3\right| \cos\phi_{23}$ | | |
| $\tilde{\mathcal{O}}^{\mathrm{IVb}}_{1+} := \frac{1}{2}\left(\mathcal{O}^{\mathrm{IV}}_{s,1} - \mathcal{O}^{\mathrm{IV}}_{s,2}\right) = \left|t_5\right| \left|t_8\right| \sin\phi_{58} + \left|t_6\right| \left|t_7\right| \sin\phi_{67}$ | | |
| $\tilde{\mathcal{O}}^{\mathrm{IVb}}_{1-} := \frac{1}{2}\left(\mathcal{O}^{\mathrm{IV}}_{s,3} - \mathcal{O}^{\mathrm{IV}}_{s,4}\right) = \left|t_5\right| \left|t_8\right| \sin\phi_{58} - \left|t_6\right| \left|t_7\right| \sin\phi_{67}$ | IVb | $\{\phi_{58}, \phi_{67}\}$ |
| $\tilde{\mathcal{O}}^{\mathrm{IVb}}_{2+} := \frac{1}{2}\left(\mathcal{O}^{\mathrm{IV}}_{c,1} - \mathcal{O}^{\mathrm{IV}}_{c,2}\right) = \left|t_5\right| \left|t_8\right| \cos\phi_{58} + \left|t_6\right| \left|t_7\right| \cos\phi_{67}$ | | |
| $\tilde{\mathcal{O}}^{\mathrm{IVb}}_{2-} := \frac{1}{2}\left(\mathcal{O}^{\mathrm{IV}}_{c,3} - \mathcal{O}^{\mathrm{IV}}_{c,4}\right) = \left|t_5\right| \left|t_8\right| \cos\phi_{58} - \left|t_6\right| \left|t_7\right| \cos\phi_{67}$ | | |
| $\tilde{\mathcal{O}}^{\mathrm{Va}}_{1+} := \frac{1}{2}\left(\mathcal{O}^{\mathrm{V}}_{s,1} + \mathcal{O}^{\mathrm{V}}_{s,2}\right) = \left|t_1\right| \left|t_5\right| \sin\phi_{15} + \left|t_2\right| \left|t_6\right| \sin\phi_{26}$ | | |
| $\tilde{\mathcal{O}}^{\mathrm{Va}}_{1-} := \frac{1}{2}\left(\mathcal{O}^{\mathrm{V}}_{s,3} + \mathcal{O}^{\mathrm{V}}_{s,4}\right) = \left|t_1\right| \left|t_5\right| \sin\phi_{15} - \left|t_2\right| \left|t_6\right| \sin\phi_{26}$ | Va | $\{\phi_{15}, \phi_{26}\}$ |
| $\tilde{\mathcal{O}}^{\mathrm{Va}}_{2+} := \frac{1}{2}\left(\mathcal{O}^{\mathrm{V}}_{c,1} + \mathcal{O}^{\mathrm{V}}_{c,2}\right) = \left|t_1\right| \left|t_5\right| \cos\phi_{15} + \left|t_2\right| \left|t_6\right| \cos\phi_{26}$ | | |
| $\tilde{\mathcal{O}}^{\mathrm{Va}}_{2-} := \frac{1}{2}\left(\mathcal{O}^{\mathrm{V}}_{c,3} + \mathcal{O}^{\mathrm{V}}_{c,4}\right) = \left|t_1\right| \left|t_5\right| \cos\phi_{15} - \left|t_2\right| \left|t_6\right| \cos\phi_{26}$ | | |
| $\tilde{\mathcal{O}}^{\mathrm{Vb}}_{1+} := \frac{1}{2}\left(\mathcal{O}^{\mathrm{V}}_{s,1} - \mathcal{O}^{\mathrm{V}}_{s,2}\right) = \left|t_3\right| \left|t_7\right| \sin\phi_{37} + \left|t_4\right| \left|t_8\right| \sin\phi_{48}$ | | |
| $\tilde{\mathcal{O}}^{\mathrm{Vb}}_{1-} := \frac{1}{2}\left(\mathcal{O}^{\mathrm{V}}_{s,3} - \mathcal{O}^{\mathrm{V}}_{s,4}\right) = \left|t_3\right| \left|t_7\right| \sin\phi_{37} - \left|t_4\right| \left|t_8\right| \sin\phi_{48}$ | Vb | $\{\phi_{37}, \phi_{48}\}$ |
| $\tilde{\mathcal{O}}^{\mathrm{Vb}}_{2+} := \frac{1}{2}\left(\mathcal{O}^{\mathrm{V}}_{c,1} - \mathcal{O}^{\mathrm{V}}_{c,2}\right) = \left|t_3\right| \left|t_7\right| \cos\phi_{37} + \left|t_4\right| \left|t_8\right| \cos\phi_{48}$ | | |
| $\tilde{\mathcal{O}}^{\mathrm{Vb}}_{2-} := \frac{1}{2}\left(\mathcal{O}^{\mathrm{V}}_{c,3} - \mathcal{O}^{\mathrm{V}}_{c,4}\right) = \left|t_3\right| \left|t_7\right| \cos\phi_{37} - \left|t_4\right| \left|t_8\right| \cos\phi_{48}$ | | |

Tables I and II. No further transformation has been applied to the diagonal observables (i.e. shape-class "I"). They are always assumed to be measured anyway.

The question is now whether one can use Nakayamas phase-fixing techniques [1] in some clever way in order to infer some complete sets composed of $2N = 16$ observables algebraically.

It is clear that an important ingredient in the following analysis are *consistency relations* among the relative phases of the different shape-classes. Generally, there exist many such relations! Here, one example for a relation that connects the (modified) shape-classes "IIa", "IIb", "VIIIa" and "VIb" is given:

$$\underbrace{\phi_{13} + \phi_{24}}_{\mathrm{IIa}} + \underbrace{\phi_{57} + \phi_{68}}_{\mathrm{IIb}} = \underbrace{\phi_{18} + \phi_{27}}_{\mathrm{VIIIa}} - \underbrace{\phi_{35} - \phi_{46}}_{\mathrm{VIb}}, \tag{17}$$

It is tentative to try to extend Nakayamas [1] treatment of the $\mathbf{(2+1+1)}$-case in single-meson photoproduction to the corresponding case of $\mathbf{(2+2+1+1+1+1)}$ observables in 2-meson photoproduction. This means we pick two different pairs of observables $\tilde{\mathcal{O}}$ from two of the modified shape-classes shown in Tables I and II and furthermore

TABLE II. The decoupled shape-classes are collected here for the cases "VI", "VII" and "VIII".

| Observable | (Shape-) class | Relative phases |
|---|---|---|
| $\tilde{\mathcal{O}}^{\mathrm{VIa}}_{1+} := \frac{1}{2}\left(\mathcal{O}^{\mathrm{VI}}_{s,1} + \mathcal{O}^{\mathrm{VI}}_{s,2}\right) = \lvert t_1\rvert \lvert t_7\rvert \sin\phi_{17} + \lvert t_2\rvert \lvert t_8\rvert \sin\phi_{28}$ | | |
| $\tilde{\mathcal{O}}^{\mathrm{VIa}}_{1-} := \frac{1}{2}\left(\mathcal{O}^{\mathrm{VI}}_{s,3} + \mathcal{O}^{\mathrm{VI}}_{s,4}\right) = \lvert t_1\rvert \lvert t_7\rvert \sin\phi_{17} - \lvert t_2\rvert \lvert t_8\rvert \sin\phi_{28}$ | VIa | $\{\phi_{17}, \phi_{28}\}$ |
| $\tilde{\mathcal{O}}^{\mathrm{VIa}}_{2+} := \frac{1}{2}\left(\mathcal{O}^{\mathrm{VI}}_{c,1} + \mathcal{O}^{\mathrm{VI}}_{c,2}\right) = \lvert t_1\rvert \lvert t_7\rvert \cos\phi_{17} + \lvert t_2\rvert \lvert t_8\rvert \cos\phi_{28}$ | | |
| $\tilde{\mathcal{O}}^{\mathrm{VIa}}_{2-} := \frac{1}{2}\left(\mathcal{O}^{\mathrm{VI}}_{c,3} + \mathcal{O}^{\mathrm{VI}}_{c,4}\right) = \lvert t_1\rvert \lvert t_7\rvert \cos\phi_{17} - \lvert t_2\rvert \lvert t_8\rvert \cos\phi_{28}$ | | |
| $\tilde{\mathcal{O}}^{\mathrm{VIb}}_{1+} := \frac{1}{2}\left(\mathcal{O}^{\mathrm{VI}}_{s,1} - \mathcal{O}^{\mathrm{VI}}_{s,2}\right) = \lvert t_3\rvert \lvert t_5\rvert \sin\phi_{35} + \lvert t_4\rvert \lvert t_6\rvert \sin\phi_{46}$ | | |
| $\tilde{\mathcal{O}}^{\mathrm{VIb}}_{1-} := \frac{1}{2}\left(\mathcal{O}^{\mathrm{VI}}_{s,3} - \mathcal{O}^{\mathrm{VI}}_{s,4}\right) = \lvert t_3\rvert \lvert t_5\rvert \sin\phi_{35} - \lvert t_4\rvert \lvert t_6\rvert \sin\phi_{46}$ | VIb | $\{\phi_{35}, \phi_{46}\}$ |
| $\tilde{\mathcal{O}}^{\mathrm{VIb}}_{2+} := \frac{1}{2}\left(\mathcal{O}^{\mathrm{VI}}_{c,1} - \mathcal{O}^{\mathrm{VI}}_{c,2}\right) = \lvert t_3\rvert \lvert t_5\rvert \cos\phi_{35} + \lvert t_4\rvert \lvert t_6\rvert \cos\phi_{46}$ | | |
| $\tilde{\mathcal{O}}^{\mathrm{VIb}}_{2-} := \frac{1}{2}\left(\mathcal{O}^{\mathrm{VI}}_{c,3} - \mathcal{O}^{\mathrm{VI}}_{c,4}\right) = \lvert t_3\rvert \lvert t_5\rvert \cos\phi_{35} - \lvert t_4\rvert \lvert t_6\rvert \cos\phi_{46}$ | | |
| $\tilde{\mathcal{O}}^{\mathrm{VIIa}}_{1+} := \frac{1}{2}\left(\mathcal{O}^{\mathrm{VII}}_{s,1} + \mathcal{O}^{\mathrm{VII}}_{s,2}\right) = \lvert t_1\rvert \lvert t_6\rvert \sin\phi_{16} + \lvert t_2\rvert \lvert t_5\rvert \sin\phi_{25}$ | | |
| $\tilde{\mathcal{O}}^{\mathrm{VIIa}}_{1-} := \frac{1}{2}\left(\mathcal{O}^{\mathrm{VII}}_{s,3} + \mathcal{O}^{\mathrm{VII}}_{s,4}\right) = \lvert t_1\rvert \lvert t_6\rvert \sin\phi_{16} - \lvert t_2\rvert \lvert t_5\rvert \sin\phi_{25}$ | VIIa | $\{\phi_{16}, \phi_{25}\}$ |
| $\tilde{\mathcal{O}}^{\mathrm{VIIa}}_{2+} := \frac{1}{2}\left(\mathcal{O}^{\mathrm{VII}}_{c,1} + \mathcal{O}^{\mathrm{VII}}_{c,2}\right) = \lvert t_1\rvert \lvert t_6\rvert \cos\phi_{16} + \lvert t_2\rvert \lvert t_5\rvert \cos\phi_{25}$ | | |
| $\tilde{\mathcal{O}}^{\mathrm{VIIa}}_{2-} := \frac{1}{2}\left(\mathcal{O}^{\mathrm{VII}}_{c,3} + \mathcal{O}^{\mathrm{VII}}_{c,4}\right) = \lvert t_1\rvert \lvert t_6\rvert \cos\phi_{16} - \lvert t_2\rvert \lvert t_5\rvert \cos\phi_{25}$ | | |
| $\tilde{\mathcal{O}}^{\mathrm{VIIb}}_{1+} := \frac{1}{2}\left(\mathcal{O}^{\mathrm{VII}}_{s,1} - \mathcal{O}^{\mathrm{VII}}_{s,2}\right) = \lvert t_3\rvert \lvert t_8\rvert \sin\phi_{38} + \lvert t_4\rvert \lvert t_7\rvert \sin\phi_{47}$ | | |
| $\tilde{\mathcal{O}}^{\mathrm{VIIb}}_{1-} := \frac{1}{2}\left(\mathcal{O}^{\mathrm{VII}}_{s,3} - \mathcal{O}^{\mathrm{VII}}_{s,4}\right) = \lvert t_3\rvert \lvert t_8\rvert \sin\phi_{38} - \lvert t_4\rvert \lvert t_7\rvert \sin\phi_{47}$ | VIIb | $\{\phi_{38}, \phi_{47}\}$ |
| $\tilde{\mathcal{O}}^{\mathrm{VIIb}}_{2+} := \frac{1}{2}\left(\mathcal{O}^{\mathrm{VII}}_{c,1} - \mathcal{O}^{\mathrm{VII}}_{c,2}\right) = \lvert t_3\rvert \lvert t_8\rvert \cos\phi_{38} + \lvert t_4\rvert \lvert t_7\rvert \cos\phi_{47}$ | | |
| $\tilde{\mathcal{O}}^{\mathrm{VIIb}}_{2-} := \frac{1}{2}\left(\mathcal{O}^{\mathrm{VII}}_{c,3} - \mathcal{O}^{\mathrm{VII}}_{c,4}\right) = \lvert t_3\rvert \lvert t_8\rvert \cos\phi_{38} - \lvert t_4\rvert \lvert t_7\rvert \cos\phi_{47}$ | | |
| $\tilde{\mathcal{O}}^{\mathrm{VIIIa}}_{1+} := \frac{1}{2}\left(\mathcal{O}^{\mathrm{VIII}}_{s,1} + \mathcal{O}^{\mathrm{VIII}}_{s,2}\right) = \lvert t_1\rvert \lvert t_8\rvert \sin\phi_{18} + \lvert t_2\rvert \lvert t_7\rvert \sin\phi_{27}$ | | |
| $\tilde{\mathcal{O}}^{\mathrm{VIIIa}}_{1-} := \frac{1}{2}\left(\mathcal{O}^{\mathrm{VIII}}_{s,3} + \mathcal{O}^{\mathrm{VIII}}_{s,4}\right) = \lvert t_1\rvert \lvert t_8\rvert \sin\phi_{18} - \lvert t_2\rvert \lvert t_7\rvert \sin\phi_{27}$ | VIIIa | $\{\phi_{18}, \phi_{27}\}$ |
| $\tilde{\mathcal{O}}^{\mathrm{VIIIa}}_{2+} := \frac{1}{2}\left(\mathcal{O}^{\mathrm{VIII}}_{c,1} + \mathcal{O}^{\mathrm{VIII}}_{c,2}\right) = \lvert t_1\rvert \lvert t_8\rvert \cos\phi_{18} + \lvert t_2\rvert \lvert t_7\rvert \cos\phi_{27}$ | | |
| $\tilde{\mathcal{O}}^{\mathrm{VIIIa}}_{2-} := \frac{1}{2}\left(\mathcal{O}^{\mathrm{VIII}}_{c,3} + \mathcal{O}^{\mathrm{VIII}}_{c,4}\right) = \lvert t_1\rvert \lvert t_8\rvert \cos\phi_{18} - \lvert t_2\rvert \lvert t_7\rvert \cos\phi_{27}$ | | |
| $\tilde{\mathcal{O}}^{\mathrm{VIIIb}}_{1+} := \frac{1}{2}\left(\mathcal{O}^{\mathrm{VIII}}_{s,1} - \mathcal{O}^{\mathrm{VIII}}_{s,2}\right) = \lvert t_3\rvert \lvert t_6\rvert \sin\phi_{36} + \lvert t_4\rvert \lvert t_5\rvert \sin\phi_{45}$ | | |
| $\tilde{\mathcal{O}}^{\mathrm{VIIIb}}_{1-} := \frac{1}{2}\left(\mathcal{O}^{\mathrm{VIII}}_{s,3} - \mathcal{O}^{\mathrm{VIII}}_{s,4}\right) = \lvert t_3\rvert \lvert t_6\rvert \sin\phi_{36} - \lvert t_4\rvert \lvert t_5\rvert \sin\phi_{45}$ | VIIIb | $\{\phi_{36}, \phi_{45}\}$ |
| $\tilde{\mathcal{O}}^{\mathrm{VIIIb}}_{2+} := \frac{1}{2}\left(\mathcal{O}^{\mathrm{VIII}}_{c,1} - \mathcal{O}^{\mathrm{VIII}}_{c,2}\right) = \lvert t_3\rvert \lvert t_6\rvert \cos\phi_{36} + \lvert t_4\rvert \lvert t_5\rvert \cos\phi_{45}$ | | |
| $\tilde{\mathcal{O}}^{\mathrm{VIIIb}}_{2-} := \frac{1}{2}\left(\mathcal{O}^{\mathrm{VIII}}_{c,3} - \mathcal{O}^{\mathrm{VIII}}_{c,4}\right) = \lvert t_3\rvert \lvert t_6\rvert \cos\phi_{36} - \lvert t_4\rvert \lvert t_5\rvert \cos\phi_{45}$ | | |

one single observables from four of the remaining modified shape-classes.

In order to exemplify what is meant, the following set of observables, which should be able to satisfy the consistency relation (17), is considered:

$$\left\{\tilde{\mathcal{O}}^{\mathrm{IIa}}_{1+}, \tilde{\mathcal{O}}^{\mathrm{IIa}}_{2+}, \tilde{\mathcal{O}}^{\mathrm{IIb}}_{1+}, \tilde{\mathcal{O}}^{\mathrm{IIb}}_{2+}, \tilde{\mathcal{O}}^{\mathrm{VIb}}_{1+}, \tilde{\mathcal{O}}^{\mathrm{VIIIa}}_{2+}\right\}. \tag{18}$$

This set of observables corresponds, in the original, i.e. non-transformed, basis $\mathcal{O}$ to the following eight observables

$$\left\{\mathcal{O}^{\mathrm{II}}_{s,1}, \mathcal{O}^{\mathrm{II}}_{s,2}, \mathcal{O}^{\mathrm{II}}_{c,1}, \mathcal{O}^{\mathrm{II}}_{c,2}, \mathcal{O}^{\mathrm{VI}}_{s,1}, \mathcal{O}^{\mathrm{VI}}_{s,2}, \mathcal{O}^{\mathrm{VIII}}_{c,1}, \mathcal{O}^{\mathrm{VIII}}_{c,2}\right\}. \tag{19}$$

Reconsidering Tables I and II, we see that the set (18) is actually equivalent to the following set of 8 observables in the $\tilde{\mathcal{O}}$-basis, which fulfills the criterion to be a $\mathbf{(2 + 2 + 1 + 1 + 1 + 1)}$-set:

$$\left\{\tilde{\mathcal{O}}^{\mathrm{IIa}}_{1+}, \tilde{\mathcal{O}}^{\mathrm{IIa}}_{2+}, \tilde{\mathcal{O}}^{\mathrm{IIb}}_{1+}, \tilde{\mathcal{O}}^{\mathrm{IIb}}_{2+}, \tilde{\mathcal{O}}^{\mathrm{VIa}}_{1+}, \tilde{\mathcal{O}}^{\mathrm{VIb}}_{1+}, \tilde{\mathcal{O}}^{\mathrm{VIIIa}}_{2+}, \tilde{\mathcal{O}}^{\mathrm{VIIIb}}_{2+}\right\}. \tag{20}$$

It was checked numerically that this set of observables, combined with the 8 diagonal observables, is in fact complete. Thus, one of the many (!) possible examples for an absolutely minimal complete set of 16 is found. The question is now how to show algebraically that the set (18) is in fact complete. In order to do this, one has to recall some results from reference [1], specifically from the sections III and IV of Nakayamas paper.

In section III of Kanzos work [1], the discrete phase-ambiguities have been worked out explicitly for, in principle, any (2 + 2)-combination coming from 2 different shape-classes in single meson photoproduction. The ambiguities for individual relative-phases are labelled by super-scripts $\lambda, \lambda', \ldots = \pm$ on the respective variables.

We collect here the results for the shape-class $b =$ "IVa", i.e. for the relative phases $\{\phi_{14}, \phi_{23}\}$. All one has to do in order to obtain the results for a different shape-class is to replace the relevant relative phases. Thus, one can also

simply read off the possible discrete ambiguities for our "decoupled" shape-classes in 2-meson photoproduction. The discrete ambiguities are grouped into cases "(A)" and "(B)":

(A) Any pair of observable of purely imaginary-type $\left(\tilde{\mathcal{O}}^m_{1+}, \tilde{\mathcal{O}}^m_{1-}\right)$, as well as any pair of observables of purely real-type $\left(\tilde{\mathcal{O}}^m_{2+}, \tilde{\mathcal{O}}^m_{2-}\right)$ (for $m = a, b, c$) yields a 4-fold discrete phase ambiguity. For the example-case of $m =$ "IVa", these ambiguities can enter the consistency-relations for the "purely imaginary" case as follows

$$\left(\tilde{\mathcal{O}}^b_{1+}, \tilde{\mathcal{O}}^b_{1-}\right) : \begin{cases} \phi^+_{14} - \phi^+_{23} = (\alpha_{14} - \alpha_{23})\,, \\ \phi^+_{14} - \phi^-_{23} = (\alpha_{14} + \alpha_{23}) - \pi, \\ \phi^-_{14} - \phi^+_{23} = -\left[(\alpha_{14} + \alpha_{23}) - \pi\right], \\ \phi^-_{14} - \phi^-_{23} = -(\alpha_{14} - \alpha_{23})\,, \\ \\ \phi^+_{14} + \phi^+_{23} = (\alpha_{14} + \alpha_{23})\,, \\ \phi^+_{14} + \phi^-_{23} = (\alpha_{14} - \alpha_{23}) + \pi, \\ \phi^-_{14} + \phi^+_{23} = -\left[(\alpha_{14} - \alpha_{23}) - \pi\right], \\ \phi^-_{14} + \phi^-_{23} = -(\alpha_{14} + \alpha_{23})\,, \end{cases} \tag{21}$$

with $\alpha_{14}$ and $\alpha_{23}$ defined uniquely on the interval $[-\pi/2, \pi/2]$. For the "purely real" case, the ambiguities yield the following expressions in the consistency constraints

$$\left(\tilde{\mathcal{O}}^b_{2+}, \tilde{\mathcal{O}}^b_{2-}\right) : \begin{cases} \phi^+_{14} - \phi^+_{23} = (\alpha_{14} - \alpha_{23})\,, \\ \phi^+_{14} - \phi^-_{23} = (\alpha_{14} + \alpha_{23})\,, \\ \phi^-_{14} - \phi^+_{23} = -(\alpha_{14} + \alpha_{23})\,, \\ \phi^-_{14} - \phi^-_{23} = -(\alpha_{14} - \alpha_{23})\,, \\ \\ \phi^+_{14} + \phi^+_{23} = (\alpha_{14} + \alpha_{23})\,, \\ \phi^+_{14} + \phi^-_{23} = (\alpha_{14} - \alpha_{23})\,, \\ \phi^-_{14} + \phi^+_{23} = -(\alpha_{14} - \alpha_{23})\,, \\ \phi^-_{14} + \phi^-_{23} = -(\alpha_{14} + \alpha_{23})\,, \end{cases} \tag{22}$$

where in this case, the variables $\alpha_{14}$ and $\alpha_{23}$ are defined uniquely on the interval $[0, \pi]$. Hence, in Eqs. (21) and (22), the $\alpha$'s are defined uniquely on different intervals. However, this doesn't matter, since within the consistency-relations, one always compares phases from *different* shape-classes. Thus, there is no chance to confuse $\alpha$'s defined on different intervals

(B) The discrete phase-ambiguities for the "mixed" cases, i.e. all combinations that contain both an "imaginary-" and a "real-type" observable are listed in the following. These comprise the cases, for $m = a, b, c$: $\left(\tilde{\mathcal{O}}^m_{1\pm}, \tilde{\mathcal{O}}^m_{2\mp}\right) = \left(\tilde{\mathcal{O}}^m_{1+}, \tilde{\mathcal{O}}^m_{2-}\right)$ or $\left(\tilde{\mathcal{O}}^m_{1-}, \tilde{\mathcal{O}}^m_{2+}\right)$, as well as $\left(\tilde{\mathcal{O}}^m_{1\nu}, \tilde{\mathcal{O}}^m_{2\nu}\right) = \left(\tilde{\mathcal{O}}^m_{1+}, \tilde{\mathcal{O}}^m_{2+}\right)$ or $\left(\tilde{\mathcal{O}}^m_{1-}, \tilde{\mathcal{O}}^m_{2-}\right)$.

One again has to look at the cases explicitly for the shape-class, or group, $b$. For the first two cases, the discrete ambiguity is two-fold:

$$\left(\tilde{\mathcal{O}}^b_{1-}, \tilde{\mathcal{O}}^b_{2-}\right) : \begin{cases} \phi^\lambda_{14} - \phi^\lambda_{23} = \lambda\,(\alpha_{14} - \alpha_{23})\,, \\ \phi^\lambda_{14} + \phi^\lambda_{23} = -2\zeta + \lambda\,(\alpha_{14} + \alpha_{23})\,, \end{cases} \tag{23}$$

$$\left(\tilde{\mathcal{O}}^b_{1+}, \tilde{\mathcal{O}}^b_{2-}\right) : \begin{cases} \phi^\lambda_{14} - \phi^\lambda_{23} = -2\zeta + \lambda\,(\alpha_{14} + \alpha_{23})\,, \\ \phi^\lambda_{14} + \phi^\lambda_{23} = \lambda\,(\alpha_{14} - \alpha_{23})\,, \end{cases} \tag{24}$$

with $\lambda = \pm$. In these equations, the quantities $\alpha_{14}$ and $\alpha_{23}$ are defined uniquely on the interval $[-\pi/2, \pi/2]$. The quantities $\zeta \equiv \zeta^b_{n\nu;n'\nu'}$ represent the *'transitional angles'*, defined in Kanzos paper [1] as the polar angle in a two-dimensional coordinate system, where $\tilde{\mathcal{O}}^b_{n\nu}$ is the $x$-coordinate and $\tilde{\mathcal{O}}^b_{n'\nu'}$ is the $y$-coordinate.

For the second pair of cases mentioned above, the discrete phase ambiguities are

$$\left(\tilde{\mathcal{O}}^b_{1+}, \tilde{\mathcal{O}}^b_{2+}\right) : \begin{cases} \phi^+_{14} - \phi^-_{23} = (\alpha_{14} - \alpha_{23}) + \pi, \\ \phi^-_{14} - \phi^+_{23} = -(\alpha_{14} - \alpha_{23}) + \pi, \\ \\ \phi^+_{14} + \phi^-_{23} = -2\zeta + (\alpha_{14} + \alpha_{23}) - \pi, \\ \phi^-_{14} + \phi^+_{23} = -2\zeta - (\alpha_{14} + \alpha_{23}) + \pi, \end{cases} \tag{25}$$

$$\left(\tilde{\mathcal{O}}^b_{1-}, \tilde{\mathcal{O}}^b_{2+}\right) : \begin{cases} \phi^+_{14} - \phi^-_{23} = -2\zeta + (\alpha_{14} + \alpha_{23}) - \pi, \\ \phi^-_{14} - \phi^+_{23} = -2\zeta - (\alpha_{14} + \alpha_{23}) + \pi, \\ \\ \phi^+_{14} + \phi^-_{23} = -(\alpha_{14} - \alpha_{23}) + \pi, \\ \phi^-_{14} + \phi^+_{23} = (\alpha_{14} - \alpha_{23}) + \pi, \end{cases} \tag{26}$$

where $\alpha_{14}$ and $\alpha_{23}$ are defined uniquely on the interval $[-\pi/2, \pi/2]$ as well.

When combining 4 observables from 2 different shape-classes, with 2 observables each, one has to be careful to check whether on the left-hand-side of the relevant consistency-relation (cf. Eq. (17)), at least one "transitional angle" $\zeta$ survives. In this way, one gets consistency relations which are all linearly independent for all cases. If not, one can in principle get linearly dependent consistency relations and therefore also at least one degenerate pair of solutions. Only the former case can yield a complete experiment, while the latter case cannot!! This point will be picked up and, hopefully, will be made more clear in the ensuing discussion.

Using these results from [1], one recognizes that the relative phases on the left-hand-side of the consistency relation (17) can appear in the following possible linear combinations

$$\phi^{\lambda}_{13} + \phi^{\lambda'}_{24} + \phi^{\lambda''}_{57} + \phi^{\lambda'''}_{68} , \tag{27}$$

where each of the four $\lambda$-variables can take two possible values, i.e. $\lambda, \ldots, \lambda''' = \pm$. Therefore, there exists a 16-fold discrete phase-ambiguity for the expression (27). The question is now what happens to the right-hand side of the consistency-relation (17).

Next, the derivation performed in section IV of reference [1] is adapted to the current problem. In order to do this, one writes down the observables from the shape-classes "VIa/b" and "VIIIa/b" contained in the set (20):

$$\tilde{\mathcal{O}}^{\mathrm{VIa}}_{1+} = B_{17} \sin\phi_{17} + B_{28} \sin\phi_{28}, \tag{28}$$

$$\tilde{\mathcal{O}}^{\mathrm{VIb}}_{1+} = B_{35} \sin\phi_{35} + B_{46} \sin\phi_{46}, \tag{29}$$

$$\tilde{\mathcal{O}}^{\mathrm{VIIIa}}_{2+} = B_{18} \cos\phi_{18} + B_{27} \cos\phi_{27}, \tag{30}$$

$$\tilde{\mathcal{O}}^{\mathrm{VIIIb}}_{2+} = B_{36} \cos\phi_{36} + B_{45} \cos\phi_{45}, \tag{31}$$

where the following notation according to Nakayama [1] was introduced: $B_{ij} := |t_i|\,|t_j|$.

First one needs additional auxilary conditions among the relative-phases. The first goal is, for example, to eliminate the relative phases contained in the observable $\tilde{\mathcal{O}}^{\mathrm{VIIIb}}_{2+}$, since the latter does not appear in the consistency relation (17). One can introduce the following auxilary conditions for the two relative phases that appear in this particular observable:

$$\underbrace{\phi_{36}}_{\mathrm{VIIIb}} = -\underbrace{\phi_{13} - \phi_{68}}_{\mathrm{II}} + \underbrace{\phi_{18}}_{\mathrm{VIIIa}} , \tag{32}$$

$$\underbrace{\phi_{45}}_{\mathrm{VIIIb}} = -\underbrace{\phi_{24} - \phi_{57}}_{\mathrm{II}} + \underbrace{\phi_{27}}_{\mathrm{VIIIa}} . \tag{33}$$

In doing a similar thing as Kanzo has done in equation (52) of his paper [1], one is able to eliminate the relative phases of $\tilde{\mathcal{O}}^{\mathrm{VIIIb}}_{2+}$ in favor of quantities that belong to the shape-class "II", about which we know the ambiguities (cf. equation (27)), as well as quantities belonging to the observable $\tilde{\mathcal{O}}^{\mathrm{VIIIa}}_{2+}$. This will turn out to be invaluable in the tedious derivation which now follows.

Plugging the relations (32) and (33) into the definition (31) and using addition-theorems for sine and cosine, one arrives at the following expression:

$$\tilde{\mathcal{O}}^{\mathrm{VIIIb}}_{2+} = B_{36} c_{13,68} \cos\phi_{18} + B_{45} c_{24,57} \cos\phi_{27} \tag{34}$$

$$- B_{36} s_{13,68} \sin\phi_{18} - B_{45} s_{24,57} \sin\phi_{27}, \tag{35}$$

where the following trigonometric functions, which contain only information from the shape-class "II", were defined:

$$c_{13,68} := \cos\left(-\phi_{13} - \phi_{68}\right), \tag{36}$$
$$s_{13,68} := \sin\left(-\phi_{13} - \phi_{68}\right), \tag{37}$$
$$c_{24,57} := \cos\left(-\phi_{24} - \phi_{57}\right), \tag{38}$$
$$s_{24,57} := \sin\left(-\phi_{24} - \phi_{57}\right). \tag{39}$$

Actually, these four quantities also carry all the information on the discrete phase ambiguities of the relative phases from shape-class "II" (cf. equation 27). Thus one should actually write $c_{13,68}^{\left(\lambda,\ldots,\lambda'''\right)}$ instead of just $c_{13,68}$, and so on. This fact should be caped in mind, however a simplified notation avoiding the $\lambda$'s is used in the following. They will then be re-introduced later at an appropriate point.

Now, one usea the definition (30) in order to obtain an expression for $\cos\phi_{27}$:

$$\cos\phi_{27} = \frac{\tilde{\mathcal{O}}_{2+}^{\mathrm{VIIIa}} - B_{18}\cos\phi_{18}}{B_{27}} =: \xi\left(\cos\phi_{18}\right). \tag{40}$$

Furthermore, one uses the well-known connection between sine and cosine in order to eliminate the sines in the expression (35), i.e.:

$$\sin\phi_{18} = \eta_1\sqrt{1-\cos^2\phi_{18}}, \text{ and } \sin\phi_{27} = \eta_2\sqrt{1-\cos^2\phi_{27}}, \tag{41}$$

where the $\eta_{1,2}$ are sign-prefactors that can take the values $\eta_1, \eta_2 = \pm 1$.

Armed with the results (40) and (41), one can transform the observable (35) to the following expression, which depends only on $\cos\phi_{18}$:

$$\tilde{\mathcal{O}}_{2+}^{\mathrm{VIIIb}} = B_{36}c_{13,68}\cos\phi_{18} + B_{45}c_{24,57}\xi\left(\cos\phi_{18}\right) - B_{36}s_{13,68}\eta_1\sqrt{1-\cos^2\phi_{18}} - B_{45}s_{24,57}\eta_2\sqrt{1-\xi^2\left(\cos\phi_{18}\right)}. \tag{42}$$

One isolates the terms with square-roots on one side of the equality-sign

$$B_{36}s_{13,68}\eta_1\sqrt{1-\cos^2\phi_{18}} + B_{45}s_{24,57}\eta_2\sqrt{1-\xi^2\left(\cos\phi_{18}\right)} = B_{36}c_{13,68}\cos\phi_{18} + B_{45}c_{24,57}\xi\left(\cos\phi_{18}\right) - \tilde{\mathcal{O}}_{2+}^{\mathrm{VIIIb}}, \tag{43}$$

and then square the whole equation, which leads to (remembering $\eta_1^2 = \eta_2^2 = +1$):

$$\begin{aligned} 2B_{36}B_{45}s_{13,68}s_{24,57}\eta_1\eta_2\sqrt{1-\cos^2\phi_{18}}\sqrt{1-\xi^2\left(\cos\phi_{18}\right)} \\ = \Big(B_{36}c_{13,68}\cos\phi_{18} + B_{45}c_{24,57}\xi\left(\cos\phi_{18}\right) - \tilde{\mathcal{O}}_{2+}^{\mathrm{VIIIb}}\Big)^2 \\ + B_{36}^2 s_{13,68}^2\left(\cos^2\phi_{18} - 1\right) + B_{45}^2 s_{24,57}^2\left[\xi^2\left(\cos\phi_{18}\right) - 1\right]. \end{aligned} \tag{44}$$

Squaring the equation for a second consecutive time, one obtains

$$\begin{aligned} 4B_{36}^2B_{45}^2s_{13,68}^2s_{24,57}^2\left(1-\cos^2\phi_{18}\right)\left(1-\xi^2\left[\cos\phi_{18}\right]\right) \\ = \Big\{\Big(B_{36}c_{13,68}\cos\phi_{18} + B_{45}c_{24,57}\xi\left(\cos\phi_{18}\right) - \tilde{\mathcal{O}}_{2+}^{\mathrm{VIIIb}}\Big)^2 \\ + B_{36}^2 s_{13,68}^2\left(\cos^2\phi_{18} - 1\right) + B_{45}^2 s_{24,57}^2\left[\xi^2\left(\cos\phi_{18}\right) - 1\right]\Big\}^2. \end{aligned} \tag{45}$$

This highly formidable equation now has to be solved for $\cos\phi_{18}$. The general form of equation (45) is that of a polynomial-equation of fourth order (or a "quartic" equation) in $\cos\phi_{18}$:

$$a_4\cos^4\phi_{18} + a_3\cos^3\phi_{18} + a_2\cos^2\phi_{18} + a_1\cos\phi_{18} + a_0 = 0. \tag{46}$$

One can determine closed expressions for $a_0, \ldots, a_4$ by using Mathematica and substituting the definition (40) back into (45). They read

$$\begin{aligned} a_4 = -\frac{1}{B_{27}^4}\Big\{ B_{18}^4B_{45}^4s_{24,57}^4 + 2B_{18}^2B_{45}^2s_{24,57}^2(B_{18}B_{45}c_{24,57} + B_{27}B_{36}(s_{13,68} - c_{13,68})) \\ \times(B_{18}B_{45}c_{24,57} - B_{27}B_{36}(c_{13,68} + s_{13,68})) \\ + \left((B_{27}B_{36}c_{13,68} - B_{18}B_{45}c_{24,57})^2 + B_{27}^2B_{36}^2s_{13,68}^2\right)^2\Big\}, \end{aligned} \tag{47}$$

$$a_3 = \frac{4}{B_{27}^4}\Big\{\Big(B_{18}^3 B_{45}^4 \tilde{\mathcal{O}}_{2+}^{\mathrm{VIIIa}} s_{24,57}^4 + B_{18} B_{45}^2 s_{24,57}^2 \Big((B_{27}B_{36}c_{13,68} - B_{18}B_{45}c_{24,57}) \times (B_{18}B_{27}\tilde{\mathcal{O}}_{2+}^{\mathrm{VIIIb}} - 2B_{18}B_{45}c_{24,57}\tilde{\mathcal{O}}_{2+}^{\mathrm{VIIIa}} + B_{27}B_{36}c_{13,68}\tilde{\mathcal{O}}_{2+}^{\mathrm{VIIIa}}) - B_{27}^2 B_{36}^2 \tilde{\mathcal{O}}_{2+}^{\mathrm{VIIIa}} s_{13,68}^2\Big) + (B_{27}\tilde{\mathcal{O}}_{2+}^{\mathrm{VIIIb}} - B_{45}c_{24,57}\tilde{\mathcal{O}}_{2+}^{\mathrm{VIIIa}}) \times (B_{27}B_{36}c_{13,68} - B_{18}B_{45}c_{24,57})\Big((B_{27}B_{36}c_{13,68} - B_{18}B_{45}c_{24,57})^2 + B_{27}^2 B_{36}^2 s_{13,68}^2\Big)\Big)\Big\}, \quad (48)$$

$$a_2 = \frac{2}{B_{27}^4}\Big\{\Big(B_{27}^2 B_{45}^2 \Big(B_{18}^2 \left(c_{24,57}^2 \left(B_{45}^2 s_{24,57}^2 - 3\left[\tilde{\mathcal{O}}_{2+}^{\mathrm{VIIIb}}\right]^2\right) + B_{45}^2 s_{24,57}^4 - \left[\tilde{\mathcal{O}}_{2+}^{\mathrm{VIIIb}}\right]^2 s_{24,57}^2\right) + B_{36}^2\Big(s_{13,68}^2 (B_{18} - \tilde{\mathcal{O}}_{2+}^{\mathrm{VIIIa}})(B_{18} + \tilde{\mathcal{O}}_{2+}^{\mathrm{VIIIa}})(c_{24,57} - s_{24,57})(c_{24,57} + s_{24,57}) - c_{13,68}^2 \left[\tilde{\mathcal{O}}_{2+}^{\mathrm{VIIIa}}\right]^2 \left(3c_{24,57}^2 + s_{24,57}^2\right)\Big) - 4B_{18}B_{36}c_{13,68}\tilde{\mathcal{O}}_{2+}^{\mathrm{VIIIa}}\tilde{\mathcal{O}}_{2+}^{\mathrm{VIIIb}}\left(3c_{24,57}^2 + s_{24,57}^2\right)\Big) - 3B_{18}^2 B_{45}^4 \left[\tilde{\mathcal{O}}_{2+}^{\mathrm{VIIIa}}\right]^2 \left(c_{24,57}^2 + s_{24,57}^2\right)^2 + 2B_{27}^3 B_{36} B_{45} c_{24,57}\Big( - B_{18}B_{36}^2 c_{13,68} s_{13,68}^2 + B_{18}c_{13,68}\left(3\left[\tilde{\mathcal{O}}_{2+}^{\mathrm{VIIIb}}\right]^2 - B_{45}^2 s_{24,57}^2\right) + B_{36}\tilde{\mathcal{O}}_{2+}^{\mathrm{VIIIa}}\tilde{\mathcal{O}}_{2+}^{\mathrm{VIIIb}}\left(3c_{13,68}^2 + s_{13,68}^2\right)\Big) + 6B_{18}B_{27}B_{45}^3 c_{24,57}\tilde{\mathcal{O}}_{2+}^{\mathrm{VIIIa}}\left(c_{24,57}^2 + s_{24,57}^2\right)(B_{18}\tilde{\mathcal{O}}_{2+}^{\mathrm{VIIIb}} + B_{36}c_{13,68}\tilde{\mathcal{O}}_{2+}^{\mathrm{VIIIa}}) + B_{27}^4 B_{36}^2 \Big(B_{36}^2 c_{13,68}^2 s_{13,68}^2 + B_{36}^2 s_{13,68}^4 + B_{45}^2 s_{24,57}^2 (c_{13,68} - s_{13,68})(c_{13,68} + s_{13,68}) - 3c_{13,68}^2 \left[\tilde{\mathcal{O}}_{2+}^{\mathrm{VIIIb}}\right]^2 - \left[\tilde{\mathcal{O}}_{2+}^{\mathrm{VIIIb}}\right]^2 s_{13,68}^2\Big)\Big)\Big\}, \quad (49)$$

$$a_1 = \frac{4}{B_{27}^4}\Big\{\Big(B_{45}^2 s_{24,57}^2 \Big(B_{18}B_{27}^2 B_{36}^2 \tilde{\mathcal{O}}_{2+}^{\mathrm{VIIIa}} s_{13,68}^2 + (B_{45}c_{24,57}\tilde{\mathcal{O}}_{2+}^{\mathrm{VIIIa}} - B_{27}\tilde{\mathcal{O}}_{2+}^{\mathrm{VIIIb}}) \times \Big( - B_{18}B_{27}^2 B_{45} c_{24,57} - B_{27}\tilde{\mathcal{O}}_{2+}^{\mathrm{VIIIa}}(B_{18}\tilde{\mathcal{O}}_{2+}^{\mathrm{VIIIb}} + B_{36}c_{13,68}\tilde{\mathcal{O}}_{2+}^{\mathrm{VIIIa}}) + 2B_{18}B_{45}c_{24,57}\left[\tilde{\mathcal{O}}_{2+}^{\mathrm{VIIIa}}\right]^2 + B_{27}^3 B_{36} c_{13,68}\Big)\Big) - (B_{27}\tilde{\mathcal{O}}_{2+}^{\mathrm{VIIIb}} - B_{45}c_{24,57}\tilde{\mathcal{O}}_{2+}^{\mathrm{VIIIa}}) \times (B_{27}B_{36}c_{13,68} - B_{18}B_{45}c_{24,57})(B_{27}B_{36}s_{13,68} - B_{27}\tilde{\mathcal{O}}_{2+}^{\mathrm{VIIIb}} + B_{45}c_{24,57}\tilde{\mathcal{O}}_{2+}^{\mathrm{VIIIa}}) \times (B_{27}(B_{36}s_{13,68} + \tilde{\mathcal{O}}_{2+}^{\mathrm{VIIIb}}) - B_{45}c_{24,57}\tilde{\mathcal{O}}_{2+}^{\mathrm{VIIIa}}) + B_{18}B_{45}^4 \tilde{\mathcal{O}}_{2+}^{\mathrm{VIIIa}} s_{24,57}^4 (\tilde{\mathcal{O}}_{2+}^{\mathrm{VIIIa}} - B_{27})(B_{27} + \tilde{\mathcal{O}}_{2+}^{\mathrm{VIIIa}})\Big)\Big\}, \quad (50)$$

$$a_0 = -\frac{1}{B_{27}^4}\Big\{ - 2B_{45}^2 s_{24,57}^2 (B_{27} - \tilde{\mathcal{O}}_{2+}^{\mathrm{VIIIa}})(B_{27} + \tilde{\mathcal{O}}_{2+}^{\mathrm{VIIIa}}) \times \left(B_{27}^2 B_{36}^2 s_{13,68}^2 + (B_{45}c_{24,57}\tilde{\mathcal{O}}_{2+}^{\mathrm{VIIIa}} - B_{27}\tilde{\mathcal{O}}_{2+}^{\mathrm{VIIIb}})^2\right) + \left((B_{45}c_{24,57}\tilde{\mathcal{O}}_{2+}^{\mathrm{VIIIa}} - B_{27}\tilde{\mathcal{O}}_{2+}^{\mathrm{VIIIb}})^2 - B_{27}^2 B_{36}^2 s_{13,68}^2\right)^2 + B_{45}^4 s_{24,57}^4 \left(B_{27}^2 - \left[\tilde{\mathcal{O}}_{2+}^{\mathrm{VIIIa}}\right]^2\right)^2\Big\}. \quad (51)$$

All attempts to obtain simplified closed expressions for the roots of (46) using Mathematica have failed. Instead, the solution-theory for quaritc equations for example given in [3] shall be adopted for the ensuing discussion. The four

possible roots of the quartic equation (46) can be written in the following form

$$\cos\phi_{18,\mathrm{i}} = -\frac{a_3}{4a_4} - S + \frac{1}{2}\sqrt{-4S^2 - 2p + \frac{q}{S}}, \tag{52}$$

$$\cos\phi_{18,\mathrm{ii}} = -\frac{a_3}{4a_4} - S - \frac{1}{2}\sqrt{-4S^2 - 2p + \frac{q}{S}}, \tag{53}$$

$$\cos\phi_{18,\mathrm{iii}} = -\frac{a_3}{4a_4} + S + \frac{1}{2}\sqrt{-4S^2 - 2p - \frac{q}{S}}, \tag{54}$$

$$\cos\phi_{18,\mathrm{iv}} = -\frac{a_3}{4a_4} + S - \frac{1}{2}\sqrt{-4S^2 - 2p - \frac{q}{S}}, \tag{55}$$

where the quantities $S$, $p$ and $q$ are complicated functions of the coefficients $a_0, \ldots, a_4$ [1].

Using this, and remembering that all coefficients $a_0, \ldots, a_4$, as well as the quantities $S$, $p$ and $q$, depend on the indices $\lambda, \ldots, \lambda'''$ due to the functions $s_{13,68}$, $s_{24,57}$, $c_{13,68}$ and $c_{24,57}$ (cf. equations (36) to (39)), it is possible to write the solutions for $\cos\phi_{18}$ in the following closed form:

$$\cos\phi_{18}^{(\lambda,\ldots,\lambda''')}\left(\tilde{\eta}_1,\tilde{\eta}_2\right) = -\frac{a_3^{(\lambda,\ldots,\lambda''')}}{4a_4^{(\lambda,\ldots,\lambda''')}} - \tilde{\eta}_1 S^{(\lambda,\ldots,\lambda''')} + \tilde{\eta}_2 \frac{1}{2}\sqrt{-4\left(S^{(\lambda,\ldots,\lambda''')}\right)^2 - 2p^{(\lambda,\ldots,\lambda''')} + \tilde{\eta}_1 \frac{q^{(\lambda,\ldots,\lambda''')}}{S^{(\lambda,\ldots,\lambda''')}}}. \tag{56}$$

Here, the sign-prefactors $\tilde{\eta}_1, \tilde{\eta}_2$ can each take the values $\tilde{\eta}_1, \tilde{\eta}_2 = \pm 1$ independently. Hence, due to the possible different values of the quantities $\lambda, \ldots, \lambda'''$ and $\tilde{\eta}_1, \tilde{\eta}_2$, one has $2^6 = 16 \times 4 = 64$ possible solutions. In addition, there exist 64 possible solutions for $\cos\phi_{27}$, which can be seen by means of the identity (40).

However, in addition, since only the cosine of the relevant phase is known via equation (56), the phase $\phi_{18}$ itself suffers an additional cosine-type ambiguity, i.e.

$$\left[\phi_{18}^{(\lambda,\ldots,\lambda''')}\left(\tilde{\eta}_1,\tilde{\eta}_2\right)\right]^{\pm} = \begin{cases} +\alpha_{18}^{(\lambda,\ldots,\lambda''')}\left(\tilde{\eta}_1,\tilde{\eta}_2\right), \\ -\alpha_{18}^{(\lambda,\ldots,\lambda''')}\left(\tilde{\eta}_1,\tilde{\eta}_2\right), \end{cases} \tag{57}$$

with $\alpha_{18}^{(\lambda,\ldots,\lambda''')}\left(\tilde{\eta}_1,\tilde{\eta}_2\right)$ defined uniquely on the interval $[0,\pi]$ via the equation (56). The same additional cosine-type ambiguity exists also for the relative phase $\phi_{27}$.

Considering now the observables contained in shape-class "VI", i.e. Eqs. (28) and (29). From these two, one eliminates the observable $\tilde{\mathcal{O}}^{\mathrm{VIa}}_{1+}$, since it does not enter our consistency relation (17). One can again employ suitably chose auxilary conditions for the relative phases:

$$\underbrace{\phi_{17}}_{\mathrm{VIa}} = \underbrace{\phi_{13} + \phi_{57}}_{\mathrm{II}} + \underbrace{\phi_{35}}_{\mathrm{VIb}}, \tag{58}$$

$$\underbrace{\phi_{28}}_{\mathrm{VIa}} = \underbrace{\phi_{24} + \phi_{68}}_{\mathrm{II}} + \underbrace{\phi_{46}}_{\mathrm{VIb}}. \tag{59}$$

Then, one can follow through a very similar derivation to the one shown at length above. One then arrives at a set ambiguous solutions $\sin\phi_{35}^{(\lambda,\ldots,\lambda''')}\left(\hat{\eta}_1,\hat{\eta}_2\right)$ and $\sin\phi_{46}^{(\lambda,\ldots,\lambda''')}\left(\hat{\eta}_1,\hat{\eta}_2\right)$. Hence, the sign-prefactors $\hat{\eta}_1, \hat{\eta}_2$ can be different compared to those in (56). In addition, each of the phases $\phi_{35}$ and $\phi_{46}$ suffers a discrete phase-ambiguity of the "sine-type".

Putting everything together, one arrives at the following set of cases for the consistency relation (17):

$$\phi_{13}^{\lambda} + \phi_{24}^{\lambda'} + \phi_{57}^{\lambda''} + \phi_{68}^{\lambda'''} = \left[\phi_{18}^{(\lambda,\ldots,\lambda''')}(\tilde{\eta}_1,\tilde{\eta}_2)\right]^{\pm} + \left[\phi_{27}^{(\lambda,\ldots,\lambda''')}(\tilde{\eta}_1,\tilde{\eta}_2)\right]^{\pm} - \left[\phi_{35}^{(\lambda,\ldots,\lambda''')}(\hat{\eta}_1,\hat{\eta}_2)\right]^{\pm} - \left[\phi_{46}^{(\lambda,\ldots,\lambda''')}(\hat{\eta}_1,\hat{\eta}_2)\right]^{\pm}. \tag{60}$$

---

[1] Here, the quantities $p$ and $q$ are coefficients of the second and of the first degree respectively in the associated depressed quartic: $p = \frac{8a_4a_2 - 3a_3^2}{8a_4^2}$ and $q = \frac{a_3^3 - 4a_4a_3a_2 + 8a_4^2a_1}{8a_4^3}$. The quantity $S$ is defined as: $S = \frac{1}{2}\sqrt{-\frac{2}{3}p + \frac{1}{3a_4}\left(Q + \frac{\Delta_0}{Q}\right)}$, where $Q = \sqrt[3]{\frac{\Delta_1 + \sqrt{\Delta_1^2 - 4\Delta_0^3}}{2}}$. Finally, the 'sub-discriminants' $\Delta_0$ and $\Delta_1$ are given by: $\Delta_0 = a_2^2 - 3a_3a_1 + 12a_4a_0$ and $\Delta_1 = 2a_2^3 - 9a_3a_2a_1 + 27a_3^2a_0 + 27a_4a_1^2 - 72a_4a_2a_0$.

For the left-hand-side, one has $2^4 = 16$ possibilities, while for the right-hand-side there exist $2^4 \times 2^2 \times 2^2 \times 2 \times 2 \times 2 \times 2 = 16^2 * 16 = 4096$ possibilities.

Now, the set of observables (20) is actually a fully complete set in case one can shown that all the consistency relations encompassed by equation (60) are *linearly independent*[2]. I.e., not even a single pair of linearly dependent equations is allowed to exist!

This seems generally like an impossible task. However, in certain special cases, one can ignore the plethora of possibilities on the right-hand-side of equation (60), since the left-hand-side comes to the rescue! This is the case when one chooses the observables from the shape-class “II” in such a clever way that there remains always at least (!) one “transitional angle” $(\zeta, \zeta', ...)$ on the left-hand-side of the relation (60). In this case, linear independence is always fulfilled automatically! Thus, the following rules can be extracted:

(i) One should *only* use the combinations $\left(\tilde{\mathcal{O}}^m_{1-}, \tilde{\mathcal{O}}^m_{2-}\right)$ as well as $\left(\tilde{\mathcal{O}}^m_{1+}, \tilde{\mathcal{O}}^m_{2+}\right)$ for at least one of the cases $m =$ “IIa” or $m =$ “IIb” (cf. the consistency relations (17) and (60)). However, one suspects analyses to be more stable if one fulfills this criterion for both cases $m =$ “IIa” *and* $m =$ “IIb”.

(ii) In case the criterion from (i) is satisfied, it should in principle not matter at all which observables have been chosen for the right-hand-side of (60), i.e. from the shape-classes $m =$ “VIb” as well as $m =$ “VIIIa”. As long as the two additional observables are made sure to belong to these two shape-classes, the resulting set in the $\mathcal{O}$-basis should always be fully complete!

(iii) Since one wishes to study minimal fully complete sets in the $\mathcal{O}$-basis, one of course should make sure that the selected set of 6 from the $\tilde{\mathcal{O}}$-basis maps suitably onto a set of 8 from the $\mathcal{O}$-basis.

Furthermore, it is not difficult to infer that the procedure outlined above for the combination of shape-classes “IIa”, “IIb”, “VIb” and “VIIIa” can be generalized to other combinations of shape-classes. Thus, one can propose the following algorithm for the selection of an even larger class of complete sets of 16:

(1) One chooses 4 distinct shape-classes of observables in the $\tilde{\mathcal{O}}$-basis. These 4 distinct classes have to contain one pair of classes of the form ('$x, a$'; '$x, b$'), where $x$ can be any of the following: “III”, “IV”, ... , “VIII”.

(2) The 4 shape-classes selected above should be accepted only in case it is possible to establish a consistency relation, similar to equation (17) given above, among their respective relative phases. There exist 40 possible combinations of four decoupled shape classes fulfilling the last two requirements. They are listed in the supplementary material Figs. 1 and 2.

(3) One picks a **(2 + 2 + 1 + 1)**-combination from the four shape-classes in the $\tilde{\mathcal{O}}$-basis, where the pair of **2**'s has to be selected from the pair of classes ('$x, a$'; '$x, b$'). This **(2 + 2 + 1 + 1)**-combination in the $\tilde{\mathcal{O}}$-basis have to stems from a **(4 + 2 + 2)**-combination of 8 observables in the $\mathcal{O}$-basis.

(4) The solution-theory can in principle be constructed as done in the example discussed at length above. In particular, one has to assure that for the observables one picks, there remains at least one “translational angle” $(\zeta, \zeta', \ldots)$ on the left-hand-side of the consistency relation! This should in any case yield you a fully complete set of 16 observables!


[1] K. Nakayama, Explicit derivation of the completeness condition in pseudoscalar meson photoproduction, Phys. Rev. C **100**, 035208 (2019).

[2] Y. Wunderlich, P. Kroenert, F. Afzal, and A. Thiel, Moravcsik's theorem on complete sets of polarization observables reexamined, Phys. Rev. C **102**, 034605 (2020).

[3] I. N. Bronstein and K. A. Semendjajew, *Taschenbuch der Mathematik*, 19th ed., edited by G. Grosche and V. Ziegler (BSB B. G. Teubner Verlagsgesellschaft, Nauka-Verlag, Leipzig, Moskau, 1979).


[2] In the parlance of reference [1], one calls two equations *linearly independent* in case they can*not* be transformed into each other by using the following two possible operations:

- Multiplication by $(-1)$,
- Addition/Subtraction of multiples of $2\pi$.

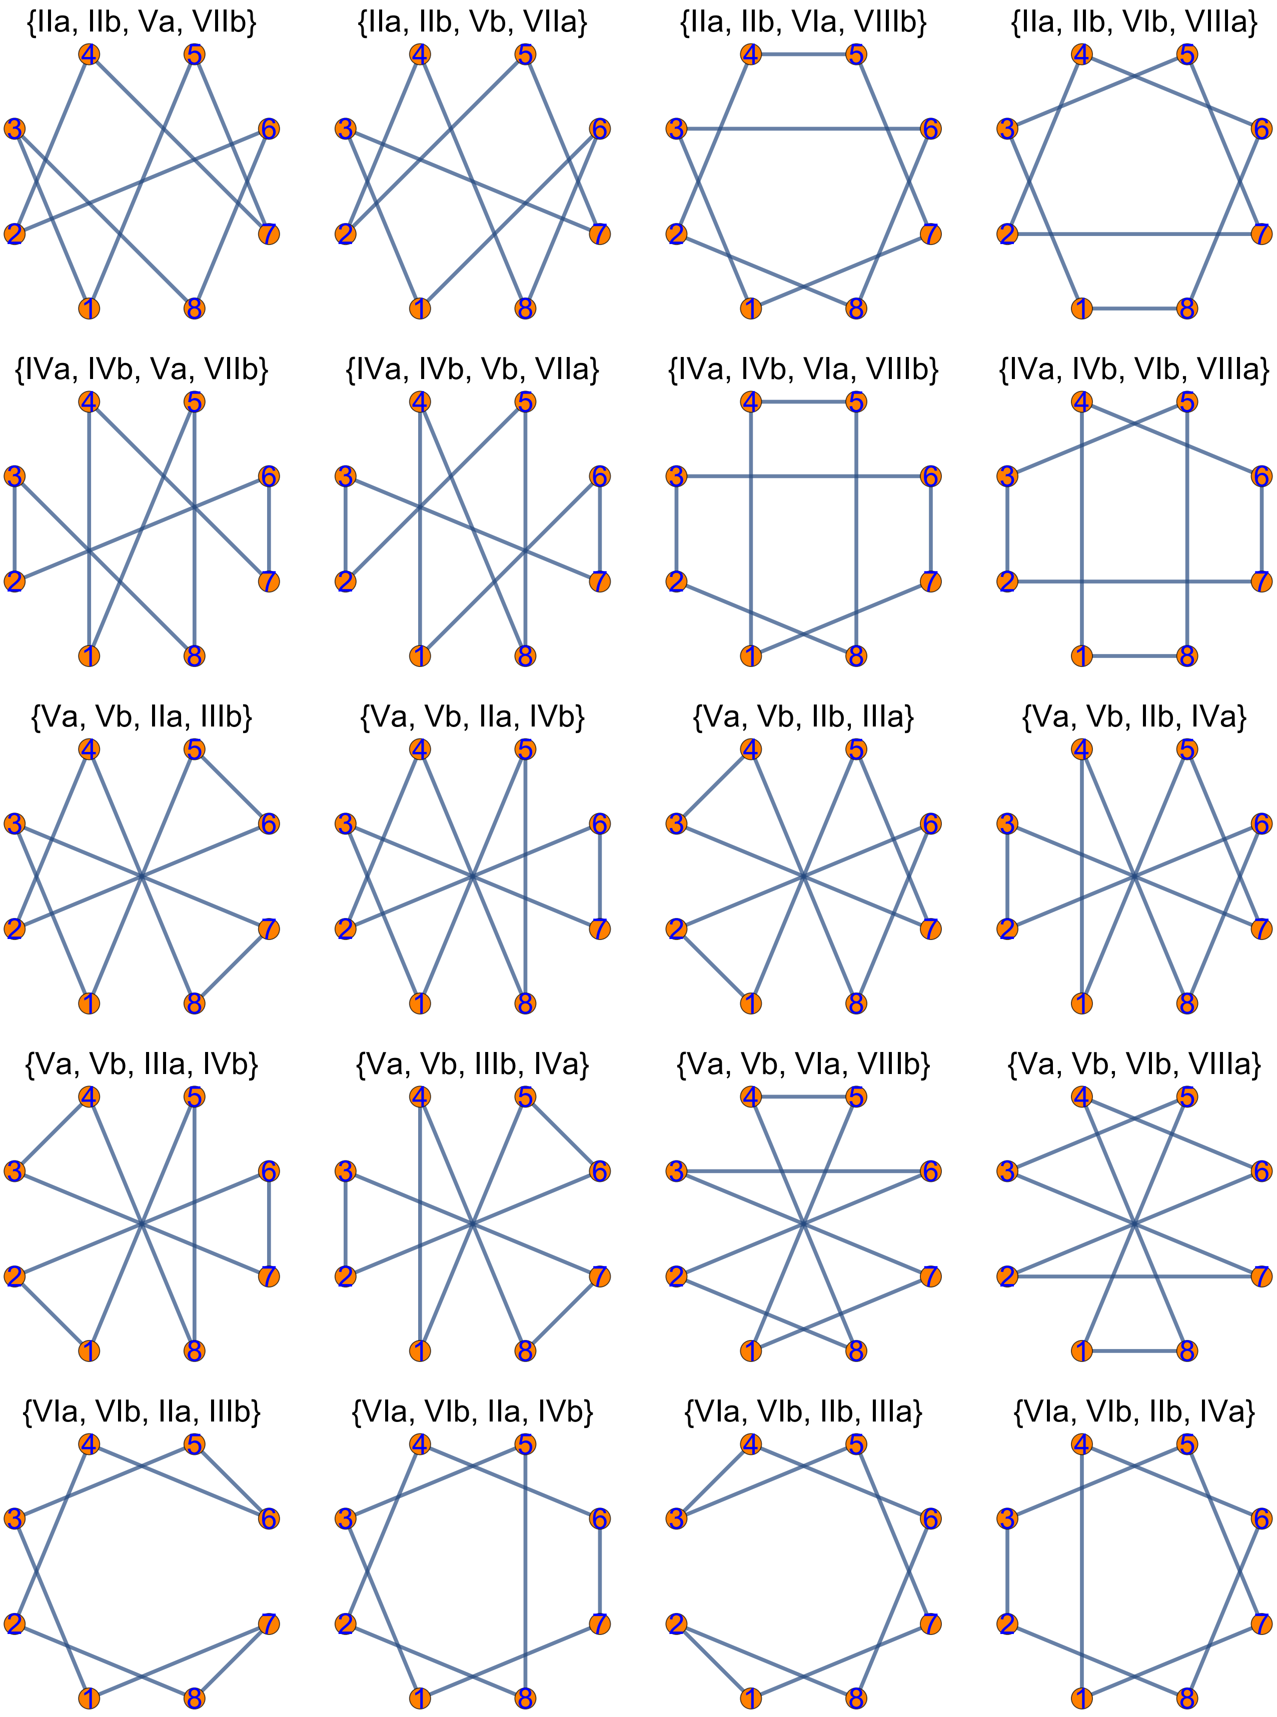


FIG. 1. Graph topologies which imply the possibility for a consistency relation and fulfilling the genral form of $\{\mathrm{Xa}, \mathrm{Xb}, \mathrm{Y}, \mathrm{Z}\}$.

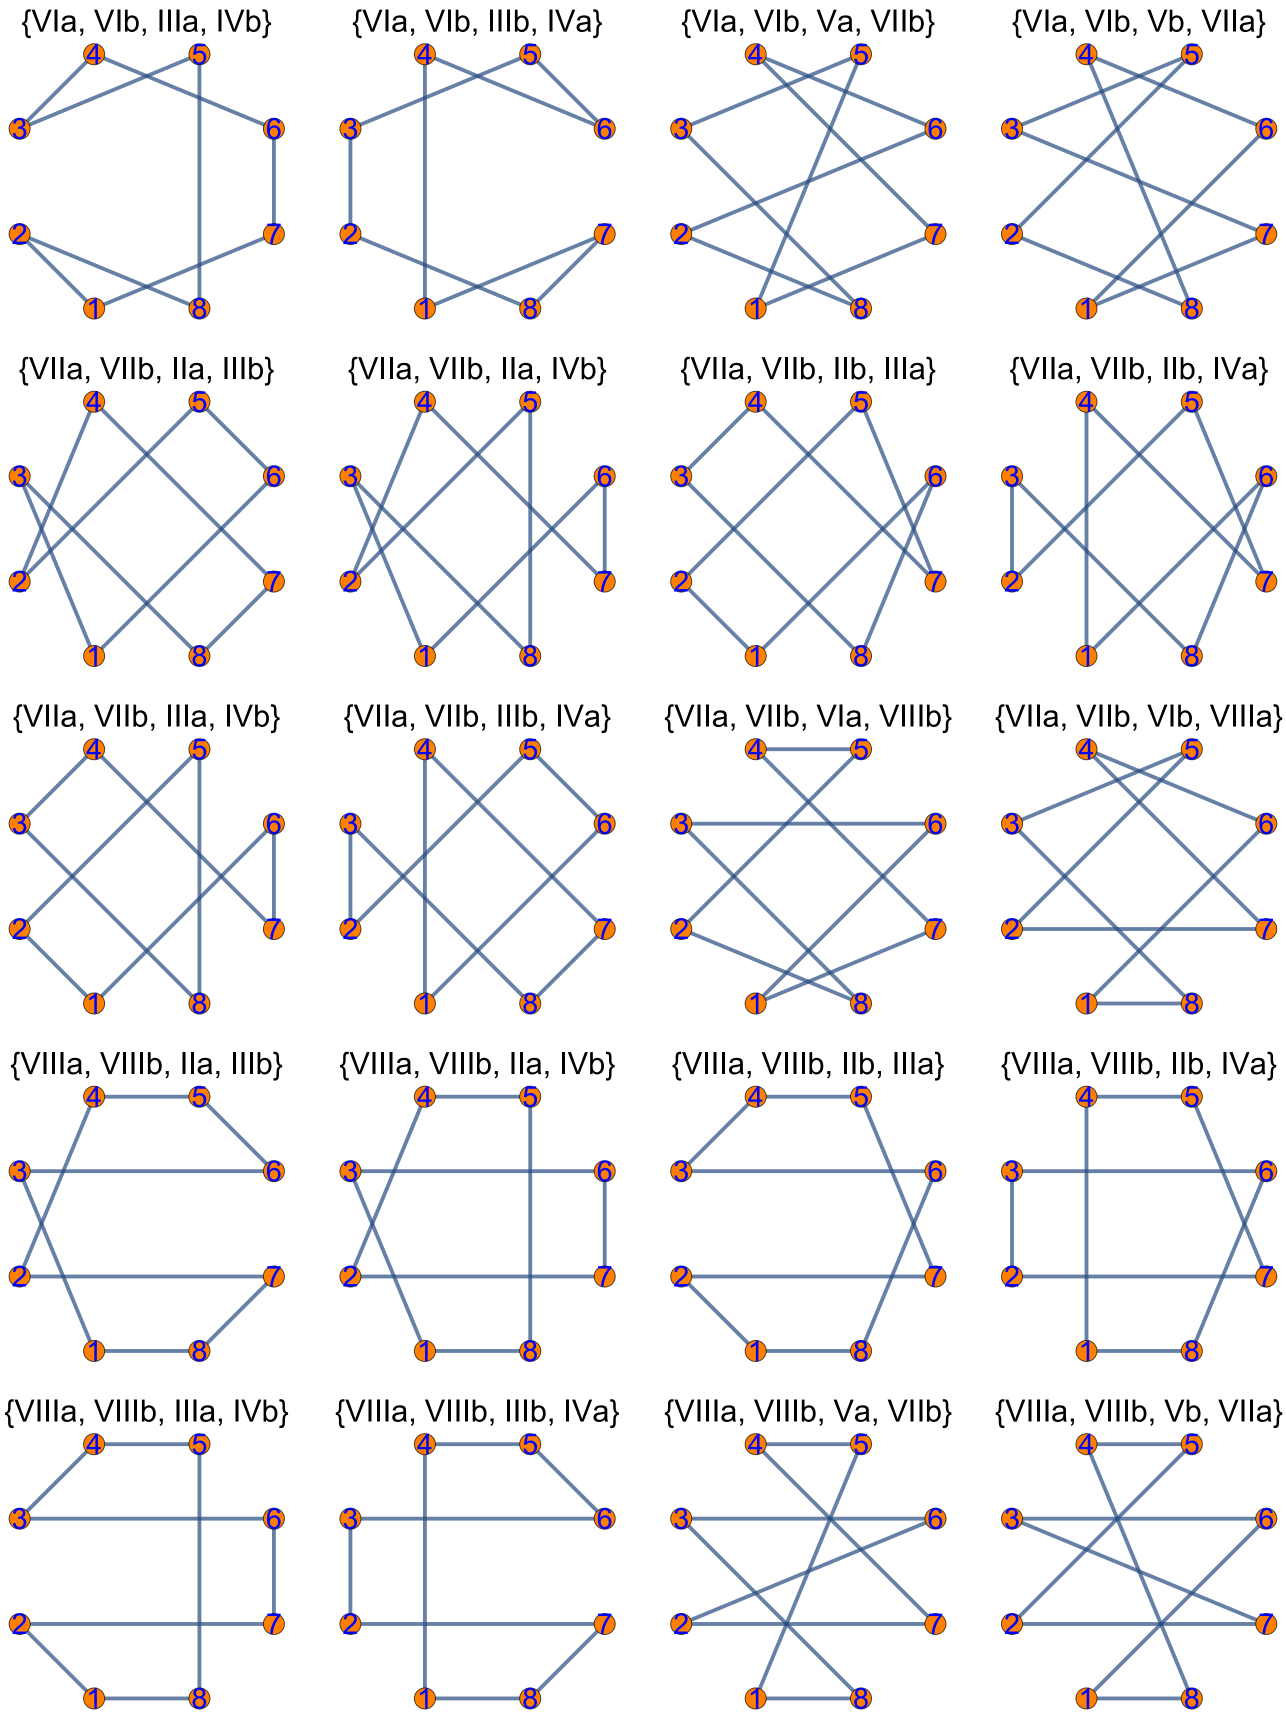


FIG. 2. Graph topologies which imply the possibility for a consistency relation and fulfilling the genral form of $\{\mathrm{Xa}, \mathrm{Xb}, \mathrm{Y}, \mathrm{Z}\}$.
